# Supplementary material for: Deep-RBF Networks for Anomaly Detection in Automotive Cyber-Physical Systems
Source: arXiv:2103.14172 source file (2021-08-23)
Supplement: Supplementary file 1 [file appendix.tex]

\newpage
\section{Source code}
https://github.com/burrussmp/Pattern\_Recognition\_Final\_Assignment.
